# Supplementary material for: Learning Spatial Pyramid Attentive Pooling in Image Synthesis and Image-to-Image Translation
Source: arXiv:1901.06322 source file (2019-01-18)
Supplement: Supplementary file 1 [file appendix.tex]

\newpage
\section{Appendix}
\subsection{Network Structures} \label{append:network_structure}
For image generation task, we used same SNDCGAN structure as \cite{kurach2018gan}, with adding A$^2$SPP model after the 64x64 feature map. Generator and Discriminator structure are shown in Table.~\ref{dcgan-gen} and Table.~\ref{dcgan-dis}. Following their annotation, convolution layer is writted as Conv(kernel, stride, pad) and the slope for leaky ReLU is 0.1. Both the generator and discriminator is added after the 64x64 feature map. 

\begin{table}[h]
\caption{SNDCGAN Generator}  \label{dcgan-gen}
\begin{center}
\begin{tabular}{c}
\hline \hline
z $\in \mathbb{R}^{128} \sim \mathcal{N}(0,1)$ \\ \hline
Linear, (h/8,w/8,512) \\ \hline
Deconv (4,2,1) BN ReLU, (h/4,w/4,256) \\ \hline
Deconv (4,2,1) BN ReLU, (h/2,w/2,128) \\ \hline
A$^2$SPP Block \\ \hline
Deconv (4,2,1) BN ReLU, (h,w,64) \\ \hline
Deconv (3,1,1) BN ReLU, Tanh, (h,w,3) \\ \hline
\hline \hline
\end{tabular}
\end{center}
\end{table}

\begin{table}[h]
\caption{SNDCGAN Discriminator}  \label{dcgan-dis}
\begin{center}
\begin{tabular}{c}
\hline \hline
RGB image $x \in \mathbb{R}^{128x128x3}$ \\ \hline
Conv(3,1,1) lReLU, (h,w,64) \\ \hline
Conv(4,2,1) lReLU, (h/2,w/2,128) \\ \hline
Conv(3,1,1) lReLU, (h/2,w/2,128) \\ \hline
Conv(4,2,1) lReLU, (h/4,w/4,256) \\ \hline
Conv(3,1,1) lReLU, (h/4,w/4,256) \\ \hline
Conv(4,2,1) lReLU, (h/8,w/8,512) \\ \hline
Conv(3,1,1) lReLU, (h/8,w/8,512) \\ \hline
Linear \\ \hline
\hline \hline
\end{tabular}
\end{center}
\end{table}

For image-to-image translation, we used the structure of CycleGAN \cite{zhu2017unpaired}. As shown in Table.~\ref{cyclegan-gen} and ~\ref{cyclegan-dis}, Convolution in generator is followed by InstanceNorm and ReLU activation. Residual block consists of two 3x3 convolutional layers with same number of filters in both layers. For 70x70 PatchGAN discriminator, Convolution is followed by InstanceNorm and LeakyReLU with slope 0.2. InstanceNorm is not used in the first Convlution layer, and final convolution is applied to produce 1-dimentional output. We add A$^2$SPP block after the 128x128 feature map.

\begin{table}[h]
\caption{CycleGAN Generator}  \label{cyclegan-gen}
\begin{center}
\begin{tabular}{c}
\hline \hline
RGB image $x \in \mathbb{R}^{256x256x3}$ \\ \hline
Conv (7, 1, 3) \\ \hline
Conv Down, 64 \\ \hline
Conv Down, 128 \\ \hline
ResBlock x 9, 128 \\ \hline
Deconv Up, 64 \\ \hline
A$^2$SPP Block \\ \hline
Deconv Up, 32 \\ \hline
Conv (7, 1, 3) \\ \hline

\hline \hline
\end{tabular}
\end{center}
\end{table}

\begin{table}[h]
\caption{CycleGAN Discriminator}  \label{cyclegan-dis}
\begin{center}
\begin{tabular}{c}
\hline \hline
RGB image $x \in \mathbb{R}^{256x256x3}$ \\ \hline
Conv (4, 2, 1), lReLU 64 \\ \hline
Conv (4, 2, 1),In lReLU 128 \\ \hline
Conv (4, 2, 1), In lReLU 256 \\ \hline
Conv (4, 1, 1), In lReLU 512 \\ \hline 
Conv (4, 1, 1) 1 \\ \hline
 
\hline \hline
\end{tabular}
\end{center}
\end{table}
